# Supplementary material for: Molecular Property Prediction: A Multilevel Quantum Interactions Modeling Perspective
Source: arXiv:1906.11081 source file (2019-06-25)
Supplement: Supplementary file 1 [file 7_appendix.tex]

\begin{figure}[tb]
    \centerline{\includesvg[width=7.5cm]{figures/count(1).svg}}
    \caption{Distribution of molecular size in two datasets.}
    \label{atomcount}
\end{figure}

There are 13 different properties in QM9. We can divide them into four groups. The first group contains five energetic properties. They are $U_0$, $U$, $H$, $G$ and $C_v$. Secondly, three related properties concern the electrons in the molecule. They consist of the energy of the electron in the highest occupied molecular orbital (HOMO) $\varepsilon_{\text{HOMO}}$, the energy in the lowest occupied molecular orbital (LUMO) $\varepsilon_{\text{LUMO}}$ and the energy difference between $\varepsilon_{\text{HOMO}}$ and $\varepsilon_{\text{LUMO}}$ that termed as gap $\Delta\varepsilon$. The third group comprises the highest fundamental vibrational frequency $\omega_1$ and the zero point vibrational energy ZPVE. The remaining properties are the electronic spatial extent $\langle R^2 \rangle$, the norm of the dipole moment $\mu$ and the norm of isotropic polarizability $\alpha$. 

Molecules in QM9 contain five kinds of elements, including Hydrogen (H), Carbon (C), Oxygen (O), Nitrogen (N), and Fluorine (F).

All of the relaxed geometries, energetic and electronic properties for all the 134k molecules are calculated by DFT at the B3LYP level of theory. The DFT error which is the empirical inaccuracy estimates of DFT can be regarded as the errors of the QM9 dataset itself \cite{faber2017prediction}. Knowing the error of the dataset helps us to evaluate the quality of models and is necessary to figure out the limitation of accuracy in this dataset. Although the QM9 dataset is limited by its accuracy, DFT errors still can provide meaningful guidance in the setting of there is no dataset with more accuracy is available temporarily. Another error level we refer to is the chemical accuracy that is generally accepted by the chemistry community as a target error. In Table \ref{error level} We present these mean absolute errors of DFT and chemical accuracy for properties in QM9.

% Table generated by Excel2LaTeX from sheet 'Sheet1'
\begin{table}[tb]
\centering

\caption{DFT Error and Chemical Accuracy For Each Property}
\begin{tabular}{llrr}
\toprule
 Property &Unit & \multicolumn{1}{l}{DFT Error} & \multicolumn{1}{l}{Chemical Accuracy} \\
\midrule
$U_0$  &eV & 0.1   & 0.043 \\
$U$  &eV & 0.1   & 0.043 \\
$G$ &eV  & 0.1   & 0.043 \\
$H$  &eV & 0.1   & 0.043 \\
$C_v$ &cal/mol K & 0.34  & 0.05 \\
 $\varepsilon_{\text{HOMO}}$  &eV & - & 0.043 \\
$\varepsilon_{\text{LUMO}}$  &eV &- & 0.043 \\
$\Delta \varepsilon$  &eV& - & 0.043 \\
$\omega_1$ &$\text{cm}^{-1} $ &  28    & 10 \\
ZPVE  &eV&  0.0097 & 0.0012 \\
$\langle R^2 \rangle $ &$\text{Bohr}^2 $&    -    & 1.2 \\
$\mu$ &Debye & 0.1   & 0.1 \\
$\alpha$ &$\text{Bohr}^3 $ & 0.4   & 0.1 \\
\bottomrule
\end{tabular}%
\label{error level}%
\end{table}%
